# Supplementary material for: Predictive Querying for Autoregressive Neural Sequence Models
Source: arXiv:2210.06464 source file (2022-11-04)
Supplement: Supplementary file 1 [file query2_is_ablation.tex]

\section{Ablation: Importance Sampling Fidelity for Long Queries}
\label{sec:is_fidelity_long_seq}

\begin{table}[H]
\begin{tabular}{lrrrrrrrr}
\toprule
{} &      \multicolumn{8}{c}{Query Sequence Length} \\
\midrule
\# Samples &      2   &      5   &      10  &      20  &      40  &      60  &      80  &      100 \\
\midrule
10    &  0.07777 &  0.10246 &  0.11593 &  0.11698 &  0.09802 &  0.10201 &  0.10335 &  0.10958 \\
30    &  0.02963 &  0.03947 &  0.04612 &  0.04419 &  0.03933 &  0.04088 &  0.04357 &  0.04604 \\
50    &  0.01701 &  0.02458 &  0.02832 &  0.02875 &  0.02656 &  0.02607 &  0.02937 &  0.03147 \\
100   &  0.00864 &  0.01296 &  0.01521 &  0.01467 &  0.01421 &  0.01600 &  0.01823 &  0.01995 \\
300   &  0.00325 &  0.00476 &  0.00534 &  0.00510 &  0.00563 &  0.00640 &  0.00777 &  0.00799 \\
500   &  0.00183 &  0.00288 &  0.00325 &  0.00303 &  0.00360 &  0.00422 &  0.00514 &  0.00551 \\
1000  &  0.00092 &  0.00140 &  0.00167 &  0.00162 &  0.00205 &  0.00229 &  0.00282 &  0.00303 \\
3000  &  0.00030 &  0.00047 &  0.00054 &  0.00058 &  0.00076 &  0.00094 &  0.00100 &  0.00111 \\
5000  &  0.00016 &  0.00027 &  0.00033 &  0.00035 &  0.00048 &  0.00056 &  0.00060 &  0.00068 \\
10000 &  0.00009 &  0.00014 &  0.00016 &  0.00017 &  0.00025 &  0.00028 &  0.00029 &  0.00035 \\
\bottomrule
\end{tabular}
\caption{Average KL Divergence (relative entropy) between pseudo-ground truth and importance sampling estimates for 100 queries taken from \textbf{Reviews} dataset. PGT was collected with an error tolerance of $\delta = 1e^{-7}$ and a maximum sample budget of $250,000$.}
\end{table}

%%%%%%%%%%%%%%%%%%%%%%%%%%%%%%%%%%%%%%%%%%%%%%%%%%%%%

\begin{table}[H]
\begin{tabular}{lrrrrrrrr}
\toprule
{} &      \multicolumn{8}{c}{Query Sequence Length} \\
\midrule
\# Samples &      2   &      5   &      10  &      20  &      40  &      60  &      80  &      100 \\
\midrule
10    &  0.24636 &  0.39938 &  0.49633 &  0.53261 &  0.50930 &  0.54033 &  0.54350 &  0.53290 \\
30    &  0.09374 &  0.16453 &  0.22747 &  0.23334 &  0.23325 &  0.24949 &  0.23519 &  0.23596 \\
50    &  0.06239 &  0.10865 &  0.14975 &  0.15478 &  0.16468 &  0.16498 &  0.15555 &  0.15791 \\
100   &  0.03151 &  0.05687 &  0.08451 &  0.09082 &  0.09006 &  0.09358 &  0.08501 &  0.08865 \\
300   &  0.00990 &  0.01970 &  0.03045 &  0.03279 &  0.03370 &  0.03335 &  0.03348 &  0.03332 \\
500   &  0.00598 &  0.01211 &  0.01817 &  0.02051 &  0.02115 &  0.02048 &  0.02005 &  0.02090 \\
1000  &  0.00311 &  0.00619 &  0.00953 &  0.01038 &  0.01092 &  0.01040 &  0.01036 &  0.01075 \\
3000  &  0.00105 &  0.00214 &  0.00317 &  0.00369 &  0.00358 &  0.00369 &  0.00373 &  0.00362 \\
5000  &  0.00064 &  0.00129 &  0.00197 &  0.00222 &  0.00220 &  0.00219 &  0.00224 &  0.00215 \\
10000 &  0.00033 &  0.00063 &  0.00098 &  0.00109 &  0.00110 &  0.00108 &  0.00110 &  0.00106 \\
\bottomrule
\end{tabular}
\caption{Average KL Divergence (relative entropy) between pseudo-ground truth and importance sampling estimates for 100 queries taken from \textbf{Shakespeare} dataset. PGT was collected with an error tolerance of $\delta = 1e^{-7}$ and a maximum sample budget of $250,000$.}
\end{table}

%%%%%%%%%%%%%%%%%%%%%%%%%%%%%%%%%%%%%%%%%%%%%%%%%%%%%

\begin{table}[H]
\begin{tabular}{lrrrrrrrr}
\toprule
{} &      \multicolumn{8}{c}{Query Sequence Length} \\
\midrule
\# Samples &      2   &      5   &      10  &      20  &      40  &      60  &      80  &      100 \\
\midrule
10    &  0.19327 &  0.37587 &  0.59260 &  0.80115 &  0.98514 &  1.09345 &  1.10783 &  1.17955 \\
30    &  0.09654 &  0.18376 &  0.28232 &  0.39400 &  0.50090 &  0.55637 &  0.55334 &  0.57453 \\
50    &  0.06370 &  0.12720 &  0.19311 &  0.26374 &  0.33748 &  0.36861 &  0.37852 &  0.39491 \\
100   &  0.03546 &  0.07182 &  0.10772 &  0.14772 &  0.18664 &  0.21176 &  0.21936 &  0.22095 \\
300   &  0.01424 &  0.02773 &  0.04329 &  0.05690 &  0.07304 &  0.07871 &  0.07949 &  0.07913 \\
500   &  0.00893 &  0.01808 &  0.02747 &  0.03640 &  0.04588 &  0.04835 &  0.04881 &  0.04880 \\
1000  &  0.00503 &  0.01018 &  0.01519 &  0.01939 &  0.02337 &  0.02429 &  0.02431 &  0.02450 \\
3000  &  0.00177 &  0.00372 &  0.00543 &  0.00687 &  0.00776 &  0.00820 &  0.00800 &  0.00811 \\
5000  &  0.00114 &  0.00232 &  0.00337 &  0.00426 &  0.00478 &  0.00492 &  0.00481 &  0.00479 \\
10000 &  0.00057 &  0.00118 &  0.00173 &  0.00212 &  0.00232 &  0.00238 &  0.00234 &  0.00236 \\
\bottomrule
\end{tabular}
\caption{Average KL Divergence (relative entropy) between pseudo-ground truth and importance sampling estimates for 100 queries taken from \textbf{MOOCs} dataset. PGT was collected with an error tolerance of $\delta = 1e^{-7}$ and a maximum sample budget of $250,000$.}
\end{table}

%%%%%%%%%%%%%%%%%%%%%%%%%%%%%%%%%%%%%%%%%%%%%%%%%%%%%

\begin{table}[H]
\begin{tabular}{lrrrrrrrr}
\toprule
{} &      \multicolumn{8}{c}{Query Sequence Length} \\
\midrule
\# Samples &      2   &      5   &      10  &      20  &      40  &      60  &      80  &      100 \\
\midrule
10    &  0.15687 &  0.27931 &  0.42376 &  0.55078 &  0.66539 &  0.74295 &  0.80917 &  0.92614 \\
30    &  0.09915 &  0.16555 &  0.24863 &  0.30317 &  0.37719 &  0.42402 &  0.43524 &  0.48099 \\
50    &  0.07670 &  0.12103 &  0.17425 &  0.21881 &  0.26294 &  0.30259 &  0.31926 &  0.33962 \\
100   &  0.05122 &  0.08178 &  0.11541 &  0.13693 &  0.16299 &  0.18352 &  0.19909 &  0.21223 \\
300   &  0.02402 &  0.03915 &  0.05160 &  0.06097 &  0.07237 &  0.08005 &  0.08406 &  0.09038 \\
500   &  0.01683 &  0.02707 &  0.03383 &  0.04074 &  0.04713 &  0.05202 &  0.05514 &  0.05796 \\
1000  &  0.00988 &  0.01540 &  0.01941 &  0.02236 &  0.02558 &  0.02821 &  0.03003 &  0.03123 \\
3000  &  0.00389 &  0.00579 &  0.00715 &  0.00832 &  0.00950 &  0.01043 &  0.01074 &  0.01122 \\
5000  &  0.00244 &  0.00357 &  0.00445 &  0.00513 &  0.00591 &  0.00641 &  0.00652 &  0.00699 \\
10000 &  0.00124 &  0.00187 &  0.00224 &  0.00261 &  0.00300 &  0.00323 &  0.00336 &  0.00356 \\
\bottomrule
\end{tabular}
\caption{Average KL Divergence (relative entropy) between pseudo-ground truth and importance sampling estimates for 100 queries taken from \textbf{Apps} dataset. PGT was collected with an error tolerance of $\delta = 1e^{-7}$ and a maximum sample budget of $250,000$.}
\end{table}
