# Supplementary material for: Predictive Querying for Autoregressive Neural Sequence Models
Source: arXiv:2210.06464 source file (2022-11-04)
Supplement: Supplementary file 2 [file OLD_Markov_appendix.tex]

\emph{This can easily go in an Appendix if we need space, but I think some readers will appreciate making connections with traditional sequence models; and its also useful for us to precisely establish  the exponential complexity for the RNN case. Note that the big O terms below need to be checked, they could quite easily be off.}

We can characterize queries as being either finite-horizon (up to step $k$, e.g., Query 3) or infinite horizon (e.g., Query 4). It is instructive to compare the complexity of  computing these types of queries exactly for each of a Markov chain and a standard AR RNN.


For a Markov chain the transition probabilities (between symbols) are fixed (homogeneous) and stored in a $V^m \times V$ matrix, where $m$ is the order of the Markov chain. For an RNN we can think of  effective transition probabilities, e.g., the probability of symbol $a$ being followed by symbol $b$. For the RNN these are not fixed but are a function of the real-valued hidden state $h$ at each step, which in turn is a function of the history of the sequence up to that point. 

\emph{We could, as a simple case for illustration, walk through the the computation involved in  computing the symbol distribution $k$-steps ahead for an RNN (Query 2)}

We can make some basic statements on time-complexity in general:
\begin{itemize}
\item For 1st order Markov chains (m=1)
\begin{itemize}
 \item finite horizon: $ O(k V^2)$ 
 \item infinite horizon: $O( V^3 )$ based on inverting a $V \times V$ matrix (e.g., the fundamental matrix): need a reference on this, including for the $a$ before $b$ query.
\end{itemize}
\item Sidenote: for mth-order Markov chains with $V^m \times  V$ transition matrix
\begin{itemize}
 \item finite horizon: $O(k V^{(m(k-1))} )$ (I think)
 \item infinite horizon: probably something related to generating the pseudo-inverse  of a $ V^m  \times V$ matrix, which will likely be something between $O(V^3)$ and $O( V^3m)$.
\end{itemize}
  
\item For standard AR-RNN:
\begin{itemize}
 \item finite horizon: $O(V^{(k-1)})$
 \item infinite horizon: not sure how to state this since you have to let $k$ -> infinity 
\end{itemize} 

\end{itemize}

\emph{Note that complexities for the RNN and for the Markov chain are not necessarily in the same "computation units" since ``model calls" to each involve different computations: we should check in detail that the big O characterizations above are comparable (e.g., in terms of characterizing the number of floating-point operations required for each (operations that depend on $V$ or $k$ or $m$).}
 
\emph{In summary, exact querying with RNNs is NP-hard for both finite and infinite horizons, versus polynomial time for Markov chains (need to check precise terminology for NP-hardness). This is pretty obvious but I think its worth stating precisely in the paper.}
